# Supplementary material for: Real-Time Privacy Preservation for Robot Visual Perception
Source: arXiv:2505.05519 source file (2025-05-08)
Supplement: Supplementary file 1 [file A-appendix.tex]

\newpage
\appendix

\section{Prompts for Foundation Models}
We use the prompt below to measure how well vision-language foundation models understand the privacy specification and detect private objects or behaviors.
\subsection{LLaVA}
Since video LLaVA processes a sequence of frames, we pass a video clip along with the privacy specification.
\begin{center}
\fbox{
\begin{minipage}{24em} 
Does this video satisfy the \texttt{<Privacy Specification>}?\\ 
You must answer only YES or NO.
For example:
`YES' or `NO'
\end{minipage} }
\end{center}
\subsection{GPT-4 Vision}
We pass a single frame with the prompt to the GPT-4 Vision model to identify private information specified in the privacy specification.

\begin{center}
\fbox{
\begin{minipage}{24em} 
Does this image satisfy the \texttt{<Privacy Specification>}? \\
You must answer only YES or NO. For example:
`YES' or `NO'
\end{minipage} }
\end{center}

% \section{Video Demonstrations}
% Video demonstrations on real robots and simulations with complex privacy specifications are available in the corresponding directory in the supplementary materials folder.
